# Supplementary material for: Building high accuracy emulators for scientific simulations with deep neural architecture search
Source: arXiv:2001.08055 source file (2020-10-08)
Supplement: Supplementary file 1 [file additional-results.tex]

\section{\revision{Additional results}}

\subsection{\revision{Training results}}
The plots of training and validation losses as a function of training epochs for several cases are shown in Figure \ref{fig:trainval-losses}.
The weights during training that yield the lowest validation loss were taken for the inference and presenting the results in this paper.

\begin{figure}
    \centering
    \includegraphics[width=\linewidth]{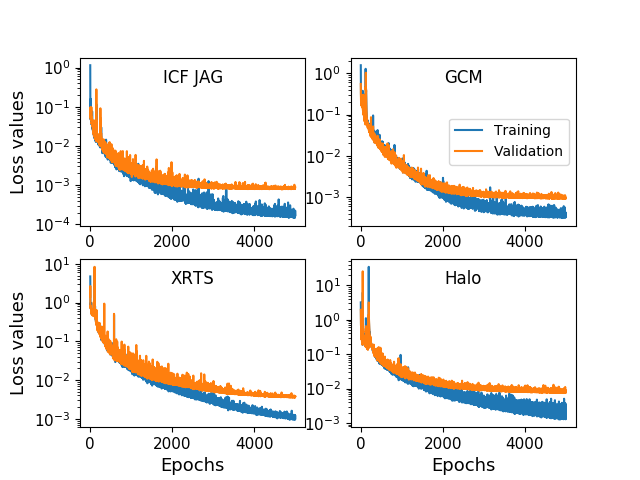}
    \caption{Loss values in training and validation datasets for a few cases.}
    \label{fig:trainval-losses}
\end{figure}

The final training, validation, and test loss for every case are presented in Table \ref{tab:testcase-lossvals-table}.
We see that most of the case has test loss not significantly different from the validation loss.
This is an exception in XES because there are a very small portion of outlier simulations that have values significantly different from the majority.
These outliers that drive up the values of the test loss value.

\begin{table*}[t!]
\begin{center}
\begin{tabular}{ |c|c|c|c|c| } 
 \hline
 \textbf{No.} &
 \textbf{Test case} & \textbf{Training loss} & \textbf{Validation loss} & \textbf{Test loss}\\
 \hline
 1 & XRTS & $7.2\times10^{-4}$ & $3.1\times10^{-3}$ & $2.8\times10^{-3}$ \\
 2 & OTS & $1.4\times10^{-4}$ & $2.3\times 10^{-4}$ & $2.4\times10^{-4}$ \\
 3 & XES & $5.2\times10^{-4}$ & $8.2\times10^{-3}$ & $1.9\times10^{-2}$ \\
 4 & ELMs & $4.0\times 10^{-4}$ & $2.0\times 10^{-3}$ & $2.1\times10^{-3}$ \\
 5 & Halo & $1.3\times10^{-3}$ & $7.2\times 10^{-3}$ & $7.7\times 10^{-3}$ \\
 6 & ICF JAG & $1.7\times10^{-4}$ & $7.8\times 10^{-4}$ & $6.6\times10^{-4}$ \\
 7 & ICF JAG Scalars & $9.1\times 10^{-6}$ & $1.2\times10^{-5}$ & $1.4\times 10^{-5}$ \\
 8 & SeisTomo & $3.5\times 10^{-3}$ & $2.7\times 10^{-2}$ & $2.4\times 10^{-2}$ \\
 9 & MOPS & $7.7\times 10^{-4}$ & $1.6\times 10^{-3}$ & $1.6\times10^{-3}$ \\
 10 & GCM & $4.1\times10^{-4}$ & $9.3\times10^{-4}$ & $9.8\times 10^{-4}$ \\
 \hline
\end{tabular}
\end{center}
\caption{\revision{Loss values for training, validation, and test datasets for each test cases.}}
\label{tab:testcase-lossvals-table}
\end{table*}

\subsection{\revision{Detailed results of DENSE and other methods on GCM}}

To show the generalization capability of DENSE, table \ref{tab:testcase-lossvals-gcm-table} presents the loss values of DENSE and non-deep learning methods for the GCM case.
Note that the random forest family methods are not included in the table because it requires memory larger than our available memory. 
The GCM case provides two dimensional outputs with only 39 data available, thus prone to overfitting.

As shown in the table, most of the methods show signs of overfitting. The sign can be seen on the loss values for training, validation, and test datasets which have very different values to each other.
SVR shows the least sign of overfitting among the non-deep learning models. However, its validation and test losses are 5 and 9 times higher than the losses achieved by DENSE.

\begin{table*}[t!]
\begin{center}
\begin{tabular}{ |c|c|c|c|c|c|c| } 
 \hline
 \textbf{No.} &
 \textbf{Method} & \textbf{Training loss} & \textbf{Validation loss} & \textbf{Test loss} & \textbf{Test/training} & \textbf{Test/validation}\\
 \hline
 1 & DENSE & $4.1\times10^{-4}$ & $9.3\times10^{-4}$ & $9.8\times 10^{-4}$ & 2.4 & 1.1 \\
 2 & Ada Boost Regressor & $6.9\times10^{-4}$ & $2.2\times 10^{-2}$ & $1.3\times 10^{-2}$ & 19 & 0.59 \\
 3 & Gradient Boosting Regressor & $6.2\times 10^{-8}$ & $1.7\times 10^{-2}$ & $1.3\times 10^{-2}$ & $2.1\times10^5$ & 0.76 \\
 4 & Gaussian Process Regressor & $2.7\times10^{-14}$ & $2.4\times10^{-2}$ & $1.1\times 10^{-2}$ & $4.1\times 10^{11}$ & 0.46 \\
 5 & Linear SVR & $9.0\times10^{-4}$ & $3.6\times 10^{-3}$ & $7.5\times 10^{-3}$ & 8.3 & 2.1\\
 6 & Nu SVR & $9.8\times10^{-4}$ & $2.6\times 10^{-3}$ & $6.0\times 10^{-3}$ & 6.1 & 2.3 \\
 7 & SVR & $3.8\times10^{-3}$ & $5.4\times 10^{-3}$ & $8.6\times 10^{-3}$ & 2.3 & 1.6 \\
 \hline
\end{tabular}
\end{center}
\caption{\revision{Loss values for training, validation, and test datasets of GCM case for DENSE and non-deep learning methods.}}
\label{tab:testcase-lossvals-gcm-table}
\end{table*}
